# Supplementary material for: Search for oscillating fundamental constants using a paired detector and vibrational spectroscopy
Source: arXiv:2502.19248 ancillary file (2025-02-26)
Supplement: Supplementary file 1 [file Supplemental.pdf]

# Supplemental Material: Search for oscillating fundamental constants using a paired detector and vibrational spectroscopy

René Oswald, Victor Vogt and Stephan Schiller

*Institut für Experimentalphysik, Heinrich-Heine-Universität Düsseldorf, 40225 Düsseldorf, Germany*

## A. Details of the apparatus

*Laser system for detector 1* A fiber laser (NKT E15) was frequency stabilized using a high-finesse optical resonator made of a NEXCERA ceramic, by means of the Pound-Drever-Hall (PDH) technique. The laser wave is coupled into an acousto-optic modulator (AOM) and split using a 99:1 fiber splitter. The smaller fraction of the light is further sent through a fiber-coupled EOM that impresses the PDH sidebands. We used sideband locking of the laser to the cavity [1, 2]. For this purpose, the phase modulator is driven by a signal of tunable frequency  $\Omega/2\pi$  in the range of 100 - 400 MHz, that is itself phase modulated at a constant frequency of 12.8 MHz. The upper laser sideband is locked to the TEM<sub>00</sub> mode of the cavity. The laser's carrier frequency could be slowly but continuously shifted relative to the cavity frequency by adjusting  $\Omega/2\pi$ , over a range of few hundred MHz. The light power within the resonator was stabilized by maintaining the light power transmitted through the resonator stable. This was accomplished by regulating appropriately the amplitude of the AOM drive signal.

*Laser system for detector 2* This laser system is similar to the system 1; however the ultrastable resonator was made out of standard ULE material.

The bandwidths of the frequency locks to the cavities are on the order of  $f_{lock} \simeq 50$  kHz. Therefore, for detection frequencies  $f > f_{lock}$  the laser frequency is determined by the laser resonator itself, as long as  $f$  is below  $f_2$ , the inverse time for sound propagation over the length of the resonator. The resonator is a section of doped silica optical fiber; from its length and speed of sound we estimate  $f_2 \simeq (6 \text{ km/s})/10 \text{ cm} \simeq 60$  kHz. In the range  $f_{lock} < f < f_2$ , the sensitivity of the laser frequency to  $m_e$  and  $\alpha$  is approximately the same as for  $f < f_{lock}$ , neglecting the fact that the index of refraction of the fiber weakly depends on  $\alpha$  and  $m_e$ . Within this approximation, we may state that for  $f > f_2$  the laser frequency is almost not affected by the fundamental constants. With  $R_\alpha^{(1)} \simeq 0$ ,  $R_{m_e}^{(1)} \simeq 0$ ,  $R_N^{(1)} = 0$  in the regime  $f > f_2$ , we obtain  $\Delta R_\alpha \simeq -2$ ,  $\Delta R_{m_e} \simeq 1.468$ ,  $\Delta R_N \simeq 0.468$ . The sensitivity to  $\alpha$  is doubled, the sensitivity to  $m_e$  is tripled, compared to the regime  $f < f_2$ . The bounds presented in sec. V of the main document ignore this effect; they are therefore conservative.

*Spectroscopy subsystems of detectors 1 and 2* In each subsystem, the laser wave was first split by a fiber splitter into a probe wave that interrogates the gas and a weaker reference wave. The probe wave was coupled out into free space and was formed into a beam of 3 mm diameter. The majority of this wave traversed a beam sampler and the 16.5 cm long gas cell. The cell contained acetylene gas under standard conditions [3]. The gas pressure was 6 Torr. The fractional absorption of the molecular resonance at our chosen wavelength of 1535.4 nm was approximately 30 %. The light transmitted through the cell was focused on detector PD1 of the balanced photodetector BPD (Femto HBPR-60K). The part of the probe wave reflected by the beam sampler was detected using photodetector PD3 in order to monitor the input power. The reference wave propagates in a fiber through an electronic variable optical attenuator (EVOA) to the second detector of the balanced photodetector, PD2. The balanced photodetector signal gain was set to 20 and a 20 MHz low-pass filter was applied directly in the BPD.

*Data acquisition* The output of each BPD was further amplified and bandpass filtered (SR560, Stanford Research Systems) with corner frequencies of usually 300 Hz and 300 kHz. The corner frequency of the lowpass was higher than the frequency range of interest, but subsequently compensated numerically. The signals of BPD 1 and 2 are recorded simultaneously by a PCIe-based 16-bit ADC card (Spectrum Instrumentation) referenced to the H-Maser. The resulting binary data was processed and analyzed after the recording by a PC with 96 GB RAM and a total of 12 TB SSD storage in RAID0 configuration. Furthermore, for monitoring purposes, in each detector the BPD output signal, both monitor signals Mon1, Mon2, and signal PD3 were recorded using a low-sampling-rate ADC card (ADC3). The digitized BPD signal was used to control the optical power level on the reference detector PD2, in order to equalize the powers on PD1 and PD2, therefore improving the suppression of technical noise. The servo was implemented using a digital 3-zone controller that adjusted the voltage applied to the EVOA approximately every 2 seconds via a DAC.

## B. Characterization of the sensitivity of the spectroscopy subsystem

The sensitivity was investigated by frequency-scanning a free-running laser around the P17 line. The laser light was split into two parts; one part was sent to a wavemeter, the other part was split in two and sent to the detectors 1 and 2. The frequency reading of the wavemeter and the monitor signals Mon1 and Mon2 of both detectors were recorded. For UDM detector 1 we show the transmission signal in Fig. 1. In the lower graph, the normalized first derivative of the transmission is shown. At the operating frequencies (blue and orange line) roughly 50 % of the incoming light is absorbed. The fractional variation of transmission  $T$  to frequency deviations  $dT/d\nu = 0.18 \text{ \%}/\text{MHz}$  was measured at PD2. During a typical experimental run, 1 mW power was detected on PD2 resulting in a sensitivity of  $D_s = 27.8 \text{ MHz/V}$  at the output of the BPD of both detectors. The gain of the amplifier (see Fig. 2 of the main document) was set to  $G_{j,m}$  in run  $m$  of detector  $j = 1, 2$ . Thus, the discriminator coefficient of a run was  $D_{j,m} = D_s/G_{j,m}$ . A typical sensitivity was  $D \approx 0.6 \text{ MHz/V}$  for a typical gain  $G \approx 50$ . The smallest frequency deviation resolvable is then presumably limited by the ADC resolution of 16 bit and its input voltage range. For a typical experiment the ADC voltage range was set to  $\pm 0.2 \text{ V}$  resulting in an presumable resolution limit of about  $6 \mu\text{Vpp}$  for a modulation signal (i.e. least significant bit, LSB), or equivalently 4 Hz pp. However, in the presence of broadband noise at the input of an ADC the resolution limit can be lower than the naive limit [4–6]. Under those conditions the inherent noise of the measurement sets the ultimate limit. In our experiment such broadband noise is indeed present. We verified that our system is able to resolve a signal of amplitude smaller than 1 LSB. In a trial experiment, we acquired  $2^{32}$  samples in the presence of noise level of 0.3 mV (standard deviation; equivalent to far more than 1 LSB) and retrieved an applied coherent signal of 80 nV amplitude. This is equivalent to  $\approx 90 \text{ MHz}$  optical frequency difference modulation amplitude. This value is sufficiently small so that it does not affect our bound, the magenta line in Fig. 4 of the main document.

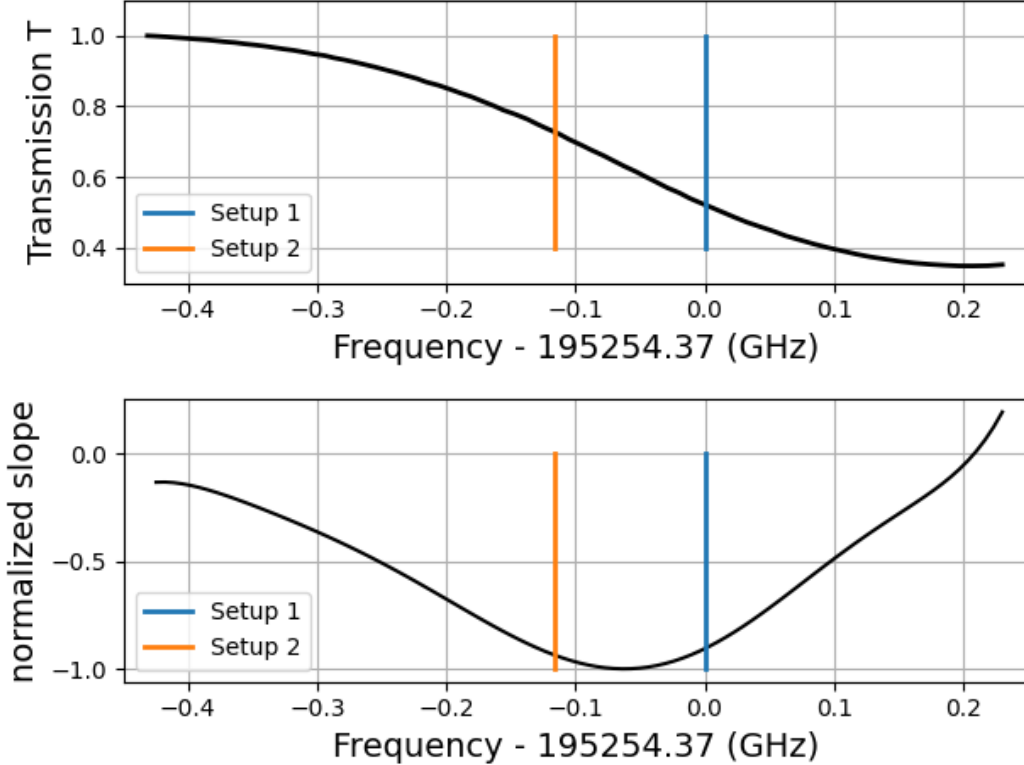

Figure 1. **Molecular discriminators and sensitivity.** Upper graph: the cell transmission on the wing of the acetylene line P17; orange and blue markers indicate the frequencies set during the actual data-taking runs. Lower graph: the normalized frequency derivative of the transmission. As can be seen, at the frequency settings employed during data taking the sensitivity of both detectors is similar.

### C. Characterization of the laser systems

The frequency noise of the lasers is a fundamental limit to the sensitivity of the detectors. We therefore determined the frequency noise directly, by analyzing the beat note between the two independent lasers 1, 2. In Figure 2 the beat note's noise power spectral density  $S_b$  is depicted in **magenta**. This noise is the sum of the power spectral densities of the individual laser frequencies, and therefore represents an upper bound to the frequency noise of each laser.

The full detector signal, as measured at ADC1 or ADC2, can also be spectrally analyzed. Let  $S_{\text{BPD}}(f)$  be the power spectral density of voltage fluctuations of a detector including the ADC during a typical experimental run. The product of its root power spectral density  $\sqrt{S_b}$  and the detector discriminator coefficient,  $D_s\sqrt{S_{\text{BPD}}}$  (**black** in the figure), can be compared with the laser frequency noise. It can be seen that over most of the studied frequency range, the laser frequency noise is more than one order smaller than the detector noise. Thus, the laser frequency noise is negligible.

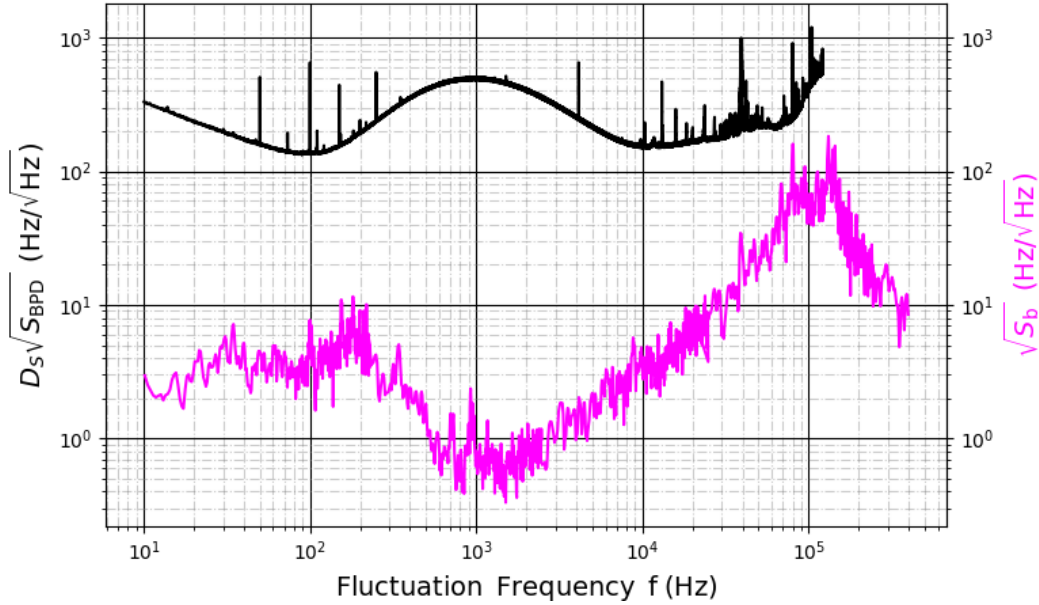

Figure 2. **Noise spectra.** **Black** : Typical total root power spectral density  $D_s\sqrt{S_{\text{BPD}}}$  of the rescaled ADC1 signal of an experimental run. This spectrum includes all noise sources. The narrow peaks are electromagnetic interference from power lines and from noise in the frequency-lock of laser 1 to its cavity. **Magenta**: Root power spectral density  $\sqrt{S_b}$  of the beat note between the two independent lasers 1 and 2. This is representative of the frequency noise of each laser.

### D. Data acquisition

Referring to Fig. 3, an experimental run (indexed by  $m$ ) consists of two simultaneously started measurements with detector 1 and 2. The BPD output voltages, amplified and bandpass filtered by amplifiers SR560, are denoted by  $x^{(m)}(t)$ . These are recorded at a sampling rate of 244 kSa/s and written onto a single file. These are the two time series of the two detectors; the identical sampling times are denoted by  $t_n$ . We chose a duration of 19 hours so that the number of samples per run,  $N$ , is a multiple of two,  $2 \times 2^{34}$  for the present choice. The recorded file is then split into two time series files, one for each detector. We also generate aggregated time series data and store them. We define aggregation as subdividing time-domain (frequency-domain) data into time (spectral) intervals of equal duration (span) and extracting from each interval the maximum, minimum, and mean value, as well as the standard deviation.

Afterwards, a FFT of the complete time series data of each detector is performed,

$$X_k^{(m)} = A \sum_{n=0}^{N-1} x^{(m)}(t_n) e^{-i2\pi \frac{nk}{N}}.$$

Here  $X_k$  is the  $k$ th component of the FFT,  $A$  is a normalization constant, and  $N$  is the number of time samples. For ease of storage of the FFT,  $A$  is set to 1. As the input time series  $x^{(m)}(t_n)$  is real valued the resulting components  $X_k$  are related by  $X_k = (X_{N-k})^*$ . In order to reduce memory usage, for further processing, only the frequency components with the index  $k$  running from 0 to  $N/2$  are stored.

Thus, without loss of information we define  $\text{HFFT}_{j,m} := \{X_k^{(m)}\}_{0 \dots N/2}$  of detector  $j$ . The  $\text{HFFT}_{j,m}$  were subsequently normalized by setting  $A$  to  $2/N$ , further corrected for the amplitude reduction introduced by the bandpass filters (SR560), and multiplied by the above mentioned discriminator coefficients  $D_{j,m}$ . The result is denoted by  $\text{FFT}_{j,m} = D_{j,m} \times \text{HFFT}_{j,m}$  and has units Hz. This is the Fourier spectrum of the variations  $\delta\nu$  of the cavity-molecular-vibration frequency difference  $\nu^{(1)} - \nu^{(2)}$ .

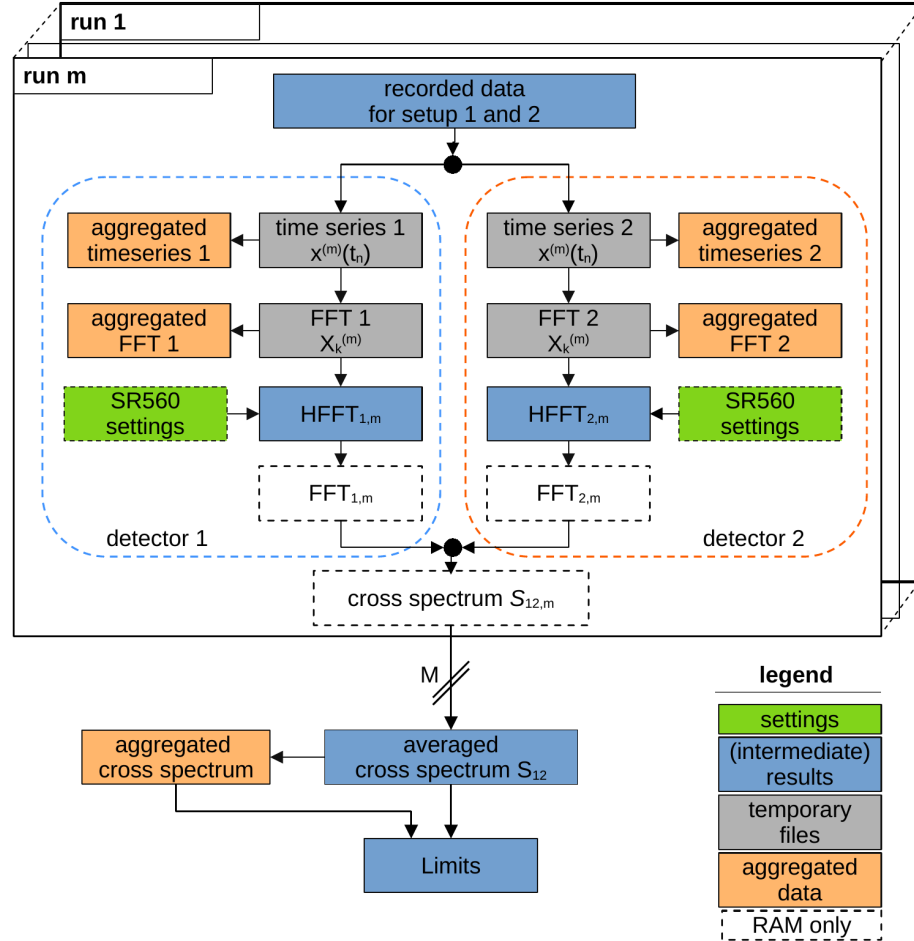

Figure 3. **Data processing flow.** **Blue** boxes: permanently saved data; **Grey** boxes: temporary data; **orange** boxes: aggregated data consisting of minimum, maximum, standard deviation and the mean value of all intervals; **green** boxes: settings relevant for data conversion; long-dashed boxes: data in RAM only.

- 
- 
- [1] J. I. Thorpe, K. Numata, and J. Livas, Laser frequency stabilization and control through offset sideband locking to optical cavities, *Opt. Express* **16**, 15980 (2008).
  - [2] A. Y. Nevsky, S. Alighanbari, Q. Chen, I. Ernsting, S. Vasilyev, S. Schiller, G. Barwood, P. Gill, N. Poli, and G. M. Tino, Robust frequency stabilization of multiple spectroscopy lasers with large and tunable offset frequencies, *Opt. Lett.* **38**, 4903 (2013).
  - [3] S. Gilbert and W. Swann, Acetylene C<sub>2</sub>H<sub>2</sub> Absorption Reference for 1510 nm to 1540 nm Wavelength Calibration - SRM 2517a, *NIST Special Publication* **260-133** (2001).
  - [4] J. Vanderkooy and S. P. Lipshitz, Resolution below the least significant bit in digital systems with dither, *Journal of The Audio Engineering Society* **32**, 106 (1984).
  - [5] W. Kester, ADC Input Noise: The Good, The Bad, and The Ugly. Is No Noise Good Noise? (Analog Devices Inc., 2005).
  - [6] J.-P. Marchal, J. Brondeau, and D. Canet, Measurement of small signals in the presence of intense peaks by fourier transform nmr, *J. Magn. Reson.* **33**, 469 (1979).
